# Supplementary material for: ProPILE: Probing Privacy Leakage in Large Language Models
Source: arXiv:2307.01881 source file (2023-07-04)
Supplement: Supplementary file 1 [file table_white-box-email.tex]

\begin{table}[]
\centering

\begin{tabular}{ccc}
\toprule
            & Likelihood & Exact match  \\
\midrule
Original    & $1.40 \times 10^{-8}$   & $0.25$             \\
Soft prompt & $1.34 \times 10^{-7}$   & $0.31$            \\
\bottomrule
\end{tabular}
\end{table}
